# Supplementary material for: Varying Manifolds in Diffusion: From Time-varying Geometries to Visual Saliency
Source: arXiv:2406.18588 source file (2024-06-07)
Supplement: Supplementary file 1 [file Appendix.tex]

%\appendix

\input{sections/8_approximation_details}
\input{sections/9_analysis_experiments}
\input{sections/10_application_details}
